# Supplementary material for: Calculation and analysis of exciton couplings via a subsystem formulation of the $GW$-Bethe-Salpeter Equation
Source: arXiv:2511.17077 ancillary file (2025-11-21)
Supplement: Supplementary file 1 [file SI.pdf]

# Supporting Information

Sarathchandra Khandavilli, Arno Förster, and Lucas Visscher\*

*Department of Chemistry and Pharmaceutical Sciences,*

*Vrije Universiteit, De Boelelaan 1108,*

*1081 HZ Amsterdam, The Netherlands*

(Dated:)

## CONTENTS

|                        |   |
|------------------------|---|
| I. Excitation Energies | 1 |
| II. Structures         | 2 |
| A. Monomer structures  | 2 |
| 1. Ethylene monomer    | 2 |
| 2. Pyrene Monomer      | 2 |
| B. chlorophyll dimer   | 4 |
| References             | 9 |

## I. EXCITATION ENERGIES

TABLE I:  $G_0W_0$  vertical excitation energies (eV) and oscillator strengths (in parentheses) for the pyrene dimers separated by 3.35 Å in the slipped configuration taken from shirai et al[1]. LE-CP results are obtained by coupling only LE states, CP results include coupling to the CT states.

| $\Omega_{S_n}^{LE}$ | $\Omega_{S_n}^{CT}$ | $\Omega_{S_n}^{LE-CP}$ | $\Omega_{S_n}^{CP}$ | $\Omega_{S_n}^{LMO}$ | NEVPT2[1]   |
|---------------------|---------------------|------------------------|---------------------|----------------------|-------------|
| 3.821 (0.00)        | 4.312 (0.03)        | 3.819(0.00)            | 3.785 (0.00)        | 3.730 (0.00)         | 3.78 (0.00) |
| 3.821 (0.00)        | 4.312 (0.03)        | 3.824 (0.00)           | 3.801 (0.00)        | 3.740 (0.00)         | 3.78 (0.00) |
| 4.064 (0.33)        | 5.080 (0.00)        | 3.989 (0.00)           | 3.962 (0.50)        | 3.870 (0.00)         | 3.91 (0.00) |
| 4.064 (0.33)        | 5.080 (0.00)        | 4.125 (0.53)           | 3.965 (0.00)        | 3.894 (0.41)         | 4.05 (0.52) |

\* l.visscher@vu.nl

## II. STRUCTURES

### A. Monomer structures

#### 1. Ethylene monomer

6

|   |             |             |             |
|---|-------------|-------------|-------------|
| C | 0.00000000  | 0.00000000  | -1.32900000 |
| C | 0.00000000  | 0.00000000  | 0.00000000  |
| H | 0.00000000  | 0.92350000  | -1.89270000 |
| H | -0.00000000 | -0.92350000 | -1.89270000 |
| H | 0.00000000  | 0.92350000  | 0.56370000  |
| H | -0.00000000 | -0.92350000 | 0.56370000  |

#### 2. Pyrene Monomer

26

|   |              |               |               |
|---|--------------|---------------|---------------|
| C | 0.0000000000 | 0.0000000000  | -0.7126637500 |
| C | 0.0000000000 | 0.0000000000  | 0.7126637500  |
| C | 0.0000000000 | -1.2379370200 | -1.4293838400 |
| C | 0.0000000000 | 1.2379370200  | -1.4293838400 |
| C | 0.0000000000 | -1.2379370200 | 1.4293838400  |
| C | 0.0000000000 | 1.2379370200  | 1.4293838400  |
| C | 0.0000000000 | -2.4642017000 | -0.6826380500 |
| C | 0.0000000000 | -1.2117807400 | -2.8362988700 |
| C | 0.0000000000 | 2.4642017000  | -0.6826380500 |
| C | 0.0000000000 | 1.2117807400  | -2.8362988700 |
| C | 0.0000000000 | -2.4642017000 | 0.6826380500  |
| C | 0.0000000000 | -1.2117807400 | 2.8362988700  |
| C | 0.0000000000 | 2.4642017000  | 0.6826380500  |
| C | 0.0000000000 | 1.2117807400  | 2.8362988700  |

|   |              |               |               |
|---|--------------|---------------|---------------|
| C | 0.0000000000 | 0.0000000000  | -3.5273899700 |
| C | 0.0000000000 | 0.0000000000  | 3.5273899700  |
| H | 0.0000000000 | -3.4066057500 | -1.2326079500 |
| H | 0.0000000000 | -2.1551541500 | -3.3848563800 |
| H | 0.0000000000 | 3.4066057500  | -1.2326079500 |
| H | 0.0000000000 | 2.1551541500  | -3.3848563800 |
| H | 0.0000000000 | -3.4066057500 | 1.2326079500  |
| H | 0.0000000000 | -2.1551541500 | 3.3848563800  |
| H | 0.0000000000 | 3.4066057500  | 1.2326079500  |
| H | 0.0000000000 | 2.1551541500  | 3.3848563800  |
| H | 0.0000000000 | 0.0000000000  | -4.6175767200 |
| H | 0.0000000000 | 0.0000000000  | 4.6175767200  |

## B. chlorophyll dimer

178

B3LYP-D3(BJ)/TZP (good numerical quality) optimized geometry

|   |             |              |             |
|---|-------------|--------------|-------------|
| C | 5.00417050  | -6.90291911  | 4.49525745  |
| C | 5.13917875  | -5.52192471  | 4.53415671  |
| C | 4.01417193  | -4.97549788  | 3.86213435  |
| H | -0.52886042 | -11.55255187 | 1.47023190  |
| H | 6.81298323  | -7.47222607  | 5.46734628  |
| H | 5.42755844  | -8.49267565  | 5.86871349  |
| H | 6.21515505  | -8.66542013  | 4.30407916  |
| H | -0.33115626 | -0.41722556  | 3.42617408  |
| H | 0.78042017  | -1.16208987  | 4.58278882  |
| H | 1.08223031  | 0.47962791   | 4.00452161  |
| H | 5.60952601  | -1.21104663  | 8.02300411  |
| H | 7.06576385  | -0.38198928  | 7.39678902  |
| H | 5.43244531  | 0.14260333   | 6.88526134  |
| C | 5.91623003  | -7.93794791  | 5.06286144  |
| H | -2.66447012 | -2.00190598  | 0.55160937  |
| H | -3.85981973 | -3.13924219  | -0.05552275 |
| H | -2.55145762 | -2.58870536  | -1.10149463 |
| H | 3.35249882  | -12.66210332 | 2.28668032  |
| H | 2.53710318  | -11.85860422 | 0.93980073  |
| H | 3.79269570  | -11.00942307 | 1.83625716  |
| C | 6.00649319  | -4.43378181  | 4.96128413  |
| O | 7.06616487  | -4.46267564  | 5.54753969  |
| C | 5.28868028  | -3.09477038  | 4.46501469  |
| H | 8.81992649  | 2.23244456   | 6.07788838  |
| C | 5.03636950  | -2.15823847  | 5.63193959  |
| O | 3.95419065  | -1.93806199  | 6.12734735  |
| O | 6.18422395  | -1.61080445  | 6.05834016  |
| C | 6.05484245  | -0.70554981  | 7.16780465  |
| C | 5.67439546  | 3.16397569   | 4.16188510  |
| C | 7.06371321  | 3.42305020   | 3.67499490  |

|    |             |              |             |
|----|-------------|--------------|-------------|
| C  | 8.17746437  | 2.85068816   | 4.13119477  |
| C  | 8.30543974  | 1.81727936   | 5.20586918  |
| H  | -0.65731794 | -1.76703249  | 1.20632117  |
| H  | -1.67764462 | -8.03854758  | 0.55891999  |
| H  | -1.08451013 | -10.37728111 | 0.28206369  |
| H  | 3.69060132  | -9.25034415  | 3.79482380  |
| H  | 3.26559531  | -0.84928892  | 3.91814148  |
| H  | 1.50141000  | -0.38358025  | 1.71095180  |
| Mg | 1.61476278  | -5.50476361  | 2.23420894  |
| H  | 5.00987476  | -1.33656584  | 2.10811366  |
| C  | 4.02721210  | -3.57210709  | 3.75760213  |
| C  | -0.11182626 | -2.66168293  | 1.47528376  |
| C  | -0.90931116 | -7.42300548  | 1.00452194  |
| C  | 3.18174000  | -8.35840720  | 3.45188330  |
| N  | 1.94628619  | -3.40960179  | 2.55541456  |
| C  | 3.04863833  | -2.83421590  | 3.13855102  |
| C  | 3.02649584  | -1.33113231  | 2.97133689  |
| C  | 1.56001225  | -1.06875016  | 2.56055084  |
| C  | 1.08023607  | -2.45322311  | 2.14651762  |
| C  | 0.71775475  | -0.50722875  | 3.71212203  |
| H  | 3.71698954  | -1.23577614  | 0.92667191  |
| C  | 4.04185173  | -0.87904858  | 1.90633595  |
| C  | 4.21820467  | 0.63427979   | 1.85599686  |
| C  | 4.95241943  | 1.17483372   | 3.06359635  |
| O  | 5.54778675  | 0.49696329   | 3.86947452  |
| O  | 4.87228582  | 2.52017771   | 3.11936303  |
| N  | -0.19098753 | -5.11136438  | 1.38333608  |
| C  | -0.70491739 | -3.88083506  | 1.10408189  |
| Mg | -1.73176748 | -6.10990336  | -3.17323392 |
| C  | -4.27545941 | -4.67543921  | -4.98371306 |
| C  | -1.94911306 | -4.01630248  | 0.37383583  |
| C  | -0.27819773 | -3.03555782  | -2.87023426 |
| C  | 0.94726082  | -7.57523704  | -1.68119890 |

|   |             |              |             |
|---|-------------|--------------|-------------|
| C | -3.02975880 | -9.25443747  | -3.91132487 |
| N | -2.23119128 | -4.13407981  | -3.83717093 |
| C | -3.37829972 | -3.76291413  | -4.49226629 |
| C | -3.52052131 | -2.25495405  | -4.51816837 |
| C | -2.08584901 | -1.79172129  | -4.17369712 |
| C | -1.47326784 | -3.04679014  | -3.56729142 |
| C | -1.30312987 | -1.32957149  | -5.40819354 |
| C | -4.56167214 | -1.81722175  | -3.47496111 |
| C | -2.15971276 | -5.37001540  | 0.20548937  |
| C | -4.83658498 | -0.31916112  | -3.47435723 |
| C | -5.62460468 | 0.11792813   | -2.25855618 |
| O | -5.76778780 | -0.54143370  | -1.25460553 |
| O | -6.13491060 | 1.35581611   | -2.43023758 |
| N | 0.02728716  | -5.42535203  | -2.41116072 |
| C | 0.42156751  | -4.12442325  | -2.32174776 |
| C | 1.66536946  | -4.03376566  | -1.58403568 |
| C | 2.00240901  | -5.32097488  | -1.21921863 |
| C | 0.97345608  | -6.19459015  | -1.77121920 |
| C | 2.40670154  | -2.77121398  | -1.30271842 |
| C | -1.05900870 | -6.05267505  | 0.87606471  |
| C | 3.11094053  | -5.80393825  | -0.41740781 |
| C | 3.91846462  | -5.09734421  | 0.38696978  |
| N | -1.15991331 | -8.06880179  | -2.83229967 |
| C | -0.02116702 | -8.45417645  | -2.18973146 |
| C | 0.04208327  | -9.89907462  | -2.11308546 |
| C | -1.09443201 | -10.37477056 | -2.72066004 |
| C | -1.83540029 | -9.21723505  | -3.18465934 |
| C | 1.16615555  | -10.67720711 | -1.51154454 |
| C | -1.48039205 | -11.80316436 | -2.94613182 |
| C | -0.99598772 | -12.34361557 | -4.29985965 |
| H | 4.80456063  | 0.92678005   | 0.98002962  |
| C | -2.80164941 | -2.87995023  | -0.07861829 |
| N | -3.24061700 | -6.85767511  | -4.28587700 |

|   |             |              |             |
|---|-------------|--------------|-------------|
| C | -3.70804866 | -8.15964392  | -4.44328189 |
| C | -4.95178914 | -8.15246496  | -5.18681711 |
| C | -5.20449508 | -6.81159376  | -5.44867230 |
| C | -4.13777237 | -6.07122940  | -4.87396575 |
| C | -5.76407933 | -9.34083284  | -5.57805593 |
| C | -6.15180841 | -5.88129713  | -6.04352569 |
| O | -7.18279203 | -6.07807781  | -6.64897848 |
| C | -5.57928935 | -4.42343052  | -5.72255939 |
| C | -5.43146689 | -3.64053860  | -7.00893531 |
| C | -3.20721890 | -6.06932744  | -0.51506561 |
| O | -4.45920567 | -3.65386544  | -7.72613703 |
| O | -6.54868225 | -2.93054109  | -7.26917130 |
| C | -6.55674691 | -2.24589142  | -8.53815127 |
| C | -6.80578211 | 1.93558316   | -1.26568302 |
| C | -5.82291060 | 2.63344845   | -0.38199249 |
| C | -5.50018807 | 2.28884035   | 0.86419318  |
| C | -6.01854182 | 1.13288876   | 1.66168365  |
| H | 0.17165971  | -2.06146633  | -2.73233892 |
| H | 1.76347661  | -8.04156219  | -1.14848697 |
| H | -3.45928740 | -10.23175387 | -4.09194605 |
| C | -4.06406693 | -5.56882143  | -1.41731974 |
| H | -3.81934067 | -1.90678795  | -5.50902648 |
| H | -2.09363490 | -0.98717457  | -3.43513580 |
| H | -5.49793208 | -2.35036002  | -3.64621476 |
| H | -4.22227982 | -2.11448695  | -2.48309884 |
| H | -3.90513616 | 0.25567930   | -3.45742487 |
| H | -5.36755830 | -0.00217481  | -4.37402782 |
| H | 3.28240717  | -6.87432415  | -0.45965965 |
| H | -1.06922797 | -12.42043768 | -2.14388408 |
| H | -2.56633023 | -11.90878695 | -2.88048410 |
| H | -6.33603949 | -3.93073154  | -5.10917733 |
| N | 1.22395862  | -7.53691008  | 2.20528518  |
| H | -7.50879470 | 2.64316754   | -1.70256963 |

|   |             |              |             |
|---|-------------|--------------|-------------|
| H | -7.35199250 | 1.15145693   | -0.75070458 |
| H | -5.34320934 | 3.50210662   | -0.82246148 |
| H | 3.81877682  | -4.03302086  | 0.53588964  |
| H | 4.70283994  | -5.59289317  | 0.94163140  |
| H | -6.63539455 | 1.48634795   | 2.49347792  |
| H | -6.59718041 | 0.43423767   | 1.06265188  |
| H | -5.18422093 | 0.58134965   | 2.10219196  |
| H | -0.26886078 | -1.09544292  | -5.15319442 |
| H | -1.76190920 | -0.43765730  | -5.83978262 |
| C | 0.12836130  | -8.12076908  | 1.64116896  |
| H | -1.29728073 | -2.11107644  | -6.17004076 |
| H | 2.15780125  | -2.38657132  | -0.31093217 |
| H | 2.16184058  | -1.99534462  | -2.02749208 |
| H | 3.48464801  | -2.93510927  | -1.33807891 |
| H | 1.42813228  | -10.29656045 | -0.52304252 |
| H | 0.90556181  | -11.73013695 | -1.40540386 |
| H | 2.06468535  | -10.62206662 | -2.13250574 |
| H | -1.29759733 | -13.38390657 | -4.43787453 |
| H | -1.40715590 | -11.75498622 | -5.12154572 |
| H | 0.09184480  | -12.29003617 | -4.36766617 |
| C | 0.19133994  | -9.55923103  | 1.80577633  |
| H | -5.99491182 | -9.96857008  | -4.71396235 |
| H | -5.22533099 | -9.96439217  | -6.29712764 |
| H | -6.69951754 | -9.02707900  | -6.03765180 |
| H | -5.73898487 | -1.52836591  | -8.58820778 |
| H | -6.45486520 | -2.96280516  | -9.35105239 |
| H | -7.51704128 | -1.74160898  | -8.58925954 |
| C | 1.35379403  | -9.82570351  | 2.48806437  |
| H | 9.11260522  | 3.16399751   | 3.67379457  |
| H | -4.77579971 | 2.91814637   | 1.37541858  |
| H | 3.26546887  | 1.16017631   | 1.76524526  |
| H | -3.28061792 | -7.13268982  | -0.31200797 |
| C | 1.99201634  | -8.54747362  | 2.74082765  |

|   |             |              |             |
|---|-------------|--------------|-------------|
| H | 1.07635651  | -11.87717727 | 2.97615094  |
| H | 2.32428580  | -11.08729565 | 3.90287177  |
| H | -1.78598754 | -10.39297859 | 1.89684739  |
| H | 5.14551225  | 4.09666364   | 4.35086462  |
| H | 5.64994805  | 2.54455745   | 5.05303299  |
| H | 7.14308289  | 4.14942691   | 2.87213824  |
| H | -4.06424319 | -4.53247422  | -1.71777693 |
| H | -4.79465897 | -6.21122014  | -1.88874709 |
| C | -0.85383228 | -10.52088460 | 1.33968246  |
| H | 8.91353425  | 0.98253268   | 4.84921169  |
| H | 5.99854348  | -2.59284916  | 3.80422644  |
| C | 1.89612413  | -11.16019706 | 2.89980154  |
| H | 7.34587640  | 1.41357833   | 5.51540917  |
| C | 2.95886715  | -11.70667031 | 1.93421852  |
| N | 3.18970485  | -5.92229222  | 3.41792275  |
| C | 3.76548074  | -7.13691850  | 3.78022533  |

- 
- [1] B. Shi, D. Nachtigallova, A. J. A. Aquino, F. B. C. Machado, and H. Lischka, Excited states and excitonic interactions in prototypic polycyclic aromatic hydrocarbon dimers as models for graphitic interactions in carbon dots, *Phys. Chem. Chem. Phys.* **21**, 9077 (2019).
